# Supplementary material for: EdiBERT, a generative model for image editing
Source: arXiv:2111.15264 source file (2022-07-21)
Supplement: Supplementary file 2 [file appendix_old.tex]

\section{Results}
\begin{table}
\centering
\begin{tabular}{l|c|c|c}
& FID & Density & Coverage\\ \hline
\multicolumn{4}{l|}{\textbf{FFHQ}} \\\hline
AR & \textbf{9.6} & 1.13 & 0.85 \\
AR + Bert 20 steps ($\star$) & 12.7 & 1.16 & \textbf{0.86} \\
AR + Bert 40 steps ($\star$) & 14.0 & \textbf{1.18} & 0.85 \\
 \hline \hline 
\multicolumn{4}{l|}{\textbf{LSUN Bedroom}} \\\hline
AR & & & \\
AR + Bert ($\star$) & & & \\ \hline \hline  
\end{tabular}
\caption{Image denoising: we improve sequences generated with the autoregressive transformer. EdiBERT improves the density (realism) without altering the coverage (diversity). \label{table:denoising}}
\end{table}


\begin{table*}
\centering
\begin{tabular}{l|c|c|c|c}
FFHQ  &  FID  & FID (n=2000) & Density & Coverage \\
VQ-GAN A.R. (k=300) & 9.6 & 27.1 & 1.13 & 0.85 \\ \hline
VQ-GAN A.R. (k=300) + BERT 2D-6 (k=800,$s_l$=16,$m_l$=4,$k_l$=10) & & 35.6 & 1.14 & 0.80 \\ 
VQ-GAN A.R. (k=300) + BERT 2D-6 (k=800,$s_l$=32,$m_l$=4,$k_l$=40) & & 33.2 & 1.01 & 0.73\\
VQ-GAN A.R. (k=300) + BERT 2D-6 (k=100,$s$=64,$m_l$=4) & & 45.3 &  &  \\
VQ-GAN A.R. (k=300) + BERT 2D-6 (k=1000,$s$=64,$m_l$=4) & & 44.5 & 0.84 & 0.66 \\\hline
VQ-GAN A.R. (k=300) + BERT 2D-6 dr (k=100,$s_l$=20,$m_l$=1,$w_k=1$) & & 30.3 & 1.10 & 0.85 \\
VQ-GAN A.R. (k=300) + BERT 2D-6 dr (k=300,$s_l$=10,$m_l$=1,$w_k=1$) & & 29.5 & 1.08 & 0.85 \\
VQ-GAN A.R. (k=300) + BERT 2D-6 dr (k=300,$s_l$=20,$m_l$=1,$w_k=4$) & & 29.3  & 1.10 & 0.85 \\
VQ-GAN A.R. (k=300) + BERT 2D-6 dr (k=400,$s_l$=10,$m_l$=1,$w_k=1$) & & 28.8  & 1.09 & 0.85 \\\hline
VQ-GAN A.R. (k=300) + BERT 2D-6 M dr (k=500,$s_l$=20,$m_l$=1,$w_k=1$,mask) & 12.8 & 28.0 & 1.16 & 0.86 \\
VQ-GAN A.R. (k=300) + BERT 2D-6 M dr (k=400,$s_l$=40,$m_l$=1,$w_k=1$,mask) &  & 29.0 & 1.18 & 0.85 \\ \hline
VQ-GAN A.R. (k=300) + BERT 2D-6 dr (k=300,$s_l$=20,$m_l$=1,$w_k=1$) & 14.7 & & 1.20 & 0.85 \\
VQ-GAN A.R. (k=300) + BERT 2D-6 dr (k=300,$s_l$=40,$m_l$=1,$w_k=1$) & 17.1 & & 1.19 & 0.83 \\ \hline

VQ-GAN A.R. (k=300) + BERT 2D-9 (k=800,$s_l$=16,$m_l$=4,$k_l$=40) & & 41.2 & 1.14 & 0.89\\ \hline
VQ-GAN A.R. (k=300) + BERT 2D-10 (k=1000,$s$=128,$m$=2) & & 29.4 & 1.14 & 0.84\\ \hline
VQ-GAN A.R. (k=300) same archi & 13.5 & 28.8 \\ \hline
VQ-GAN Bert 3 (k=200) & 57.3 & 70.4 \\
VQ-GAN Bert 2D (k=200) & 63.9 & 75.2 \\
VQ-GAN Bert 2D (k=300) & 54.3 & 67.6 \\
VQ-GAN Bert 2D-3 (k=200) & 51.8 & 65.3\\
VQ-GAN Bert 2D-3 (k=300) & 46.0 & 61.2 \\
VQ-GAN Bert 2D-3 (k=600) & 45.1 & 60.7 \\
VQ-GAN Bert 2D-3 (k=600, denoise) & 40.6 & 56.8 \\
VQ-GAN Bert 2D-3 (k=600, s=128, m=4, denoise) & 39.8 & 54.7 \\
VQ-GAN Bert 2D-6 (k=600, denoise) & 38.9 & 53.8 \\
VQ-GAN Bert 2D-6 (k=800, denoise, s=128,m=4) &  & 53.1 & 0.78 & 0.56 \\
VQ-GAN Bert 2D-6 (k=800, denoise, s=128,m=8) &  & 51.4 & 0.76 & 0.56 \\
VQ-GAN Bert 2D-6 (k=800, denoise, s=128,m=8,rdom) &  & 49.7 & 0.74 & 0.56 \\
VQ-GAN Bert 2D-6 (k=800, denoise=2, s=128,m=8,rdom) &  & 49.7 & 0.75 & 0.56 \\
VQ-GAN Bert 2D-6 (k=600, denoise=2, s=256,m=2,rdom) &  & 52.6 \\
VQ-GAN Bert 2D-6 (k=800, denoise=1, s=64,m=8,rdom, \\
$s_l$=32,$m_l$=4,$k_l$=30) &  & 55.5 & 0.79 & 0.55 \\
VQ-GAN Bert 2D-6 (k=800, denoise=1, s=64,m=8,rdom, \\
$s_l$=32,$m_l$=8,$k_l$=50) &  & 61.2 & 0.62 & 0.48\\
VQ-GAN Bert 2D-uniform-2 (k=300) &  & 70.7 \\
VQ-GAN Bert 2D-uniform-2 (k=600) &  & 72.6\\ \hline \hline
Lsun Bedroom \\ \hline
VQGAN A.R. & 4.37 & & 1.23 & 0.94\\ \hline 
Model w. Rand tokens & \\
VQGAN A.R. BERT (k=300,llk=20,wkllk=1) & 4.68 & & 1.13 & 0.93 \\ 
VQGAN A.R. BERT (k=300,llk=40,wkllk=1) &  & & 1.02 & 0.92 \\ \hline
VQGAN A.R. BERT (k=100,llk=20,wkllk=1) & 4.51  & & 1.20 & 0.94 \\
VQGAN A.R. BERT (k=200,llk=20,wkllk=1) & 4.52  & & 1.23 & 0.94 \\
VQGAN A.R. BERT (k=200,llk=20,wkllk=1) & 4.52  & & 1.23 & 0.94 \\
VQGAN A.R. BERT (k=200,llk=20,wkllk=40) & 4.53  & &  &  \\
VQGAN A.R. BERT (k=300,llk=20,wkllk=1) & 4.52  & & 1.19 & 0.93 \\
VQGAN A.R. BERT (k=500,llk=30,wkllk=10) & 4.54 & & 1.16 & 0.93 \\
VQGAN A.R. BERT (k=300,llk=40,wkllk=1) & &  & 1.19  & 0.94  \\
VQGAN A.R. BERT (k=500,llk=50,wkllk=20) & &  & 1.16   &  0.93 \\
\end{tabular}
\caption{Comparison of Auto-Regressive vs. Bert Generation. \label{table:autoregressive_vs_bert}}
\end{table*}



\begin{table*}
\centering
\begin{tabular}{l|c|c|c|}
 & masked L1 &  FID & Density\\ \hline \hline 
FFHQ: large masks \\ \hline
StyleGAN2 256 Projection & 0.0767 & 23.6 & 0.99 \\
StyleGAN2-ADA 1024 Projection & 0.0763 & 22.1 & 1.25 \\
StyleGAN+Encoder(1024) & 0.1027 & 27.9 & 1.12 \\
Co-Modulated Gans (512) & 0.0128 & 4.7 & 1.24   \\
Bert VQ-GAN 2D-6 (random mask,k=100,e=4,m=4,col=1,dil=1,rnd ord )& 0.0507 & 18.3 & 1.13 \\ 
Bert VQ-GAN 2D-6 (random mask,k=100,e=4,m=4,col=2,dil=1,rnd ord) & 0.0454 &  18.0 & 1.20\\
Bert VQ-GAN 2D-6 (random mask,k=100,e=4,m=2,col=2,dil=1,rnd ord) & 0.0453 &  18.0 & 1.23\\
Bert VQ-GAN 2D-6 (random mask,k=100,e=8,m=6,col=2,dil=1) & 0.0478 &  18.1 & 1.11\\
Bert VQ-GAN 2D-6 (random mask,k=200,e=5,m=2,col=3,dil=1) & 0.0439 &  17.8 & 1.19\\
Bert VQ-GAN 2D-10 (random mask,k=100,e=4,m=4,col=1,dil=1,rnd ord ) & 0.0420 & 21.8 & 1.21 \\
Bert VQ-GAN 2D-10 (random mask,k=100,e=4,m=4,col=2,dil=1) & 0.0412 & 22.9 & 1.09\\ \hline
Bert VQ-GAN 2D-6 M ([MASK] mask,k=100,e=1,m=1,col=0,dilM=0,dilS=1) & 0.0536 &  24.7 & 1.27 \\ 
Bert VQ-GAN 2D-6 M ([MASK] mask,k=100,e=1,m=1,col=0,dilM=0,dilS=1,random) & 0.0554 &  21.3 & 1.36 \\ 
Bert VQ-GAN 2D-6 M ([MASK] mask,k=100,e=1,m=1,col=0,dilM=0,dilS=1,prog) & 0.0554 & 22.4 & 1.31 \\  
Bert VQ-GAN 2D-6 M ([MASK] mask,k=100,e=1,m=1,col=0,dilM=0,dilS=0,random) & 0.0528 & 22.2 & 1.36 \\
Bert VQ-GAN 2D-6 M ([MASK] mask,k=100,e=1,m=1,col=4,dilM=0,dilS=1,random) & 0.0432 & 21.6 & 1.27 \\
Bert VQ-GAN 2D-6 M ([MASK],k=100,e=1,m=1,col=4,dilM=0,dilS=1,random, gsm) & 0.0449 & 21.4 & 1.27 \\
Bert VQ-GAN 2D-6 M ([MASK] mask,k=100,e=1,m=1,col=3,dilM=0,dilS=1,prog, gsm) & 0.0446 & 21.7 & 1.26 \\
Bert VQ-GAN 2D-6 M ([MASK] mask,k=100,e=2,m=1,col=3,dilM=0,dilS=1,prog, gsm) & 0.0440 & 20.8 & 1.16 \\
Bert VQ-GAN 2D-6 M ([MASK],k=100,e=2,m=1,col=3,dilM=0,dilS=1,prog, gsm, [m] 2nd ep) & 0.0422 & 22.1 & 1.23 \\
Bert VQ-GAN 2D-6 M ([MASK],k=100,e=2,m=1,col=10,dilM=0,dilS=1,prog, gsm, [m] 2nd ep) & 0.0429 & 21.5 & 1.19 \\
Bert VQ-GAN 2D-6 M ([MASK] mask,k=100,e=2,m=2,col=4,dilM=0,dilS=1,random, gsm) & 0.0464 & 20.2 & 1.18 \\
Bert VQ-GAN 2D-6 M ([MASK] mask,k=200,e=1,m=1,col=3,dilM=0,dilS=1,random, gsm) & 0.0457 & 21.8 & 1.23 \\
\hline
Bert VQ-GAN 2D-6  ([rnd] mask,k=100,e=1,m=1,col=4,dilM=0,dilS=1,prog, gsm) & 0.0415 & 18.9 & 0.93 \\
Bert VQ-GAN 2D-6  ([rnd] mask,k=100,e=2,m=1,col=4,dilM=0,dilS=1,prog, gsm) & 0.0419 & 17.4 & 1.19 \\
Bert VQ-GAN 2D-6  ([rnd] mask,k=100,e=2,m=1,col=4,dilM=0,dilS=1,prog, gsm, [rnd] 2nd ep) & 0.0419 & 16.5 & 1.22 \\
Bert VQ-GAN 2D-6  ([rnd] mask,k=100,e=4,m=1,col=4,dilM=0,dilS=1,prog, gsm, [rnd] 2nd ep) & 0.0422 & 15.8 & 1.16 \\
Bert VQ-GAN 2D-6  ([rnd] mask,k=100,e=4,m=2,col=4,dilM=0,dilS=1,rand, gausmooth) & 0.0439 & 17.6 & 1.21 \\
\hline \hline
 
FFHQ: complex masks (smooth) \\ \hline
StyleGAN2+Encoder(1024) & 0.0620 & 27.9 & 1.22 \\
StyleGAN2 Projection (256) & 0.0440 & 22.3 & 0.92 \\
StyleGAN2-ADA Projection (1024) & 0.0435 & 21.1 & 1.17 \\
Co-modulated GANs (1024) & 0.0086 & 10.3 & 1.42 \\
Bert VQ-GAN 2D-6 drM ([MASK],k=100,e=1,m=1,col=0,dilM=0,dilS=0) & 0.0409 & 25.5 & 0.96 \\ 
Bert VQ-GAN 2D-6 drM ([MASK],k=100,e=1,m=1,col=0,dilM=0,dilS=1) & 0.0444 & 26.6 & 0.97 \\ 
Bert VQ-GAN 2D-6 drM ([MASK],k=100,e=1,m=1,col=0,dilM=0,dilS=1,prog) & 0.0423 & 23.3 & 1.08 \\ 
Bert VQ-GAN 2D-6 drM ([MASK],k=100,e=1,m=1,col=0,dilM=0,dilS=1,rand) & 0.0424 & 23.3 & 1.02 \\ 
Bert VQ-GAN 2D-6 drM ([MASK],k=100,e=1,m=1,col=5,dilM=0,dilS=1,prog) & 0.0300 & 19.7 & 1.14 \\ 
Bert VQ-GAN 2D-6 drM ([MASK],k=100,e=1,m=1,col=5,dilM=0,dilS=1,random) & 0.0309 & 20.0 & 1.11 \\ 
Bert VQ-GAN 2D-6 drM ([MASK],k=100,e=2,m=1,col=4,dilM=0,dilS=1,prog,[mask] on 2nd ep.) & 0.0299 & 19.8 & 1.26 \\ 
Bert VQ-GAN 2D-6 drM ([MASK],k=50,e=2,m=1,col=4,dilM=0,dilS=1,prog,[mask] on 2nd ep.) & 0.0299 & 20.3 & 1.25 \\ \hline 
Bert VQ-GAN 2D-6 dr ([rnd],k=100,e=1,m=1,col=5,dilM=0,dilS=1,prog) & 0.0284 & 26.6 & 0.93 \\ 
Bert VQ-GAN 2D-6 dr ([rnd],k=100,e=2,m=1,col=4,dilM=0,dilS=1,prog) & 0.0288 & 24.6 & 1.07 \\ 
Bert VQ-GAN 2D-6 dr ([rnd],k=100,e=4,m=2,col=5,dilM=0,dilS=1,prog) & 0.0303 & 25.4 & 1.03 \\ 
Bert VQ-GAN 2D-6 dr ([rnd],k=100,e=2,m=1,col=4,dilM=0,dilS=1,prog, [rnd] 2nd ep) & 0.0292 & 21.5 & 1.16 \\ 


\end{tabular}
\caption{Image completion: comparison of our method vs gan-based approach on a FFHQ validation set. \label{table:comparison_bert_vs_ganbased}}
\end{table*}


\begin{comment}
\begin{table*}
\centering
\begin{tabular}{l|c|c|c|}
 & masked L1 &  FID & Density\\ \hline \hline 
FFHQ \\ \hline
Composite original & 0 & 50.9 & 1.27 / 0.11 \\
Poisson & 0.1660 & 20.9 & 0.49 / 0.22 \\
StyleGAN2 256 Projection & 0.1199 &  27.4 & 0.76 \\
StyleGAN2-ADA 1024 Projection &  \\
StyleGAN2 1024 Encoder & 0.1337 & 19.5 & 1.50 / 1.97 \\
Co-modulated GANs 512 & 0.0386 & 31.8 & 1.25 / 0.39 \\

Bert-VQ GANs MASK (e=1) & & 31.1 &  / 0.26 \\
Bert-VQ GANs MASK (e=2) & & 36.3 & / 0.18\\
Bert-VQ GANs & &  \\
Bert-VQ GANs & &  \\
 \\
\end{tabular}
\caption{Image compositing. \label{table:image_compositing}}
\end{table*}
\end{comment}


\begin{table}
\centering
\begin{tabular}{l|c|c|c|}
 & Masked L1 & FID & Density \\ \hline
FFHQ & \\\hline
StyleGAN2-encoder & 0.1491 & 31.9 & 1.17 \\
StyleGAN2-projection & 0.1141 & 29.4 & 0.97 \\
StyleGAN2-ada-projection & 0.1133 & 26.9 & 1.35 \\
Bert VQ-GAN ($\star$,k100,e2,m1,dil1,col3,rand) & 0.0555 & 19.8 & 1.13 \\
Bert VQ-GAN M ($\star$,k100,e2,m1,dil2,col3,rand) & 0.0541 & 21.3 & 1.10 \\ 
Bert VQ-GAN M ($\star$,k100,e2,m1,dil2,col3,rand) & 0.0541 & 21.2 & 1.17 \\\hline \hline 
LSUN Bedroom & \\\hline
StyleGAN-encoder & & & \\
StyleGAN-projection & & & \\
Bert VQ-GAN ($\star$) & & & \\ \hline \hline  

\end{tabular}
\caption{Image crossovers: we improve sequences generated with the auto-regressive transformer.  \label{table:crossovers_appendix}}
\end{table}


\begin{comment}
\section{Bert VQ-GAN inference: Gibbs sampling}
Gibbs sampling is a Monte-Carlo Markov Chain allowing to sample from a multi-dimensional distribution. 

A bi-directional model allows to perform an approximate Gibbs sampling. Given a sequence $s$, the Bert transformer $T_\theta$ outputs a sequence of probability distributions: $T_\theta(s) \in \mathbb{R}^{L\times N}$, where $T_\theta[i]$ is the discrete probability distribution over tokens at position i, given $s$. 

\textbf{Initialization.} Given an incomplete image $\Tilde{I}$, we use as a starting sequence $s=E(\Tilde{I})$. In image completion, we typically have $\Tilde{I} = I\times m$.

\textbf{Sampling.} We iteratively update the sequence $s$ by sampling from the transformer distribution. Given a position i that we want to re-sample, we compute $T_\theta(s)$ and sample a token according to the multinomial distribution defined by $T_\theta(s)[i]$. Contrarily to auto-regressive models, there is no pre-defined ordering of positions fixed at training and inference time. We can thus vary the ordering of positions that we re-sample. As explained below, we use a random ordering and resample multiple positions for one transformer inference.

\textbf{Faster inference via random order parallel sampling.} For a faster inference, we do want to modify several tokens for one computation $T_\theta(s)$. However, this is difficult because the modification image tokens are highly correlated. Thus, we make use of the spacial structure of images: close tokens are more correlated than distant ones. 

Let us suppose that we have an initial sequence $s^l$, and a second sequence $s^{l+1}$ obtained by modifying the token at position i in $s^l$. We can study the following divergence measure: $D (T_\theta(s^l)[j] || T_\theta(s^{l+1})[j])$, where $D$ is a divergence between distributions (\textit{e.g.} KL-divergence). When re-sampling two positions at the same time, we want to select positions $i,j$ such as  $D (T_\theta(s^l)[j] || T_\theta(s^{l+1})[j])$ is minimized. We show that this divergence tends to be minimal when i and j are distant in Figure \ref{}.  

\textbf{Mask influence.} At initialization, we downsample the mask at the same resolution than the encoding, and reshape it to a 1D sequence. We then define the set of tokens to be modified as the tokens belonging to the 1D mask. We justify this choice in Figure \ref{fig:vqgan_encoding}, where we show that the encoding of VQ-GANs is quite local. 

Depending on the task, our algorithms deals with the mask in a different manner. We split the tasks in two categories: mask-dependant or mask-independant. In mask-dependant tasks (\textit{e.g.} scribble-based editing), the user modifies a spatial area and wants its edit to be improved. In mask-independant tasks (\textit{e.g.} image completion), the user only specifies a spatial area to be replaced. For mask-dependant tasks, we use the base algorithm. For mask-independant tasks, we modify the algorithm such that the sampling is not conditioned to the masked area. 
\end{comment}
